# Supplementary material for: Simultaneous computation of dynamical and equilibrium information using a weighted ensemble of trajectories
Source: arXiv:1210.3094 source file (2014-07-05)
Supplement: Supplementary file 1 [file SuppInfo3.pdf]

# Simultaneous computation of dynamical and equilibrium information using a weighted ensemble of trajectories

Ernesto Suárez<sup>1†</sup>, Steven Lettieri<sup>1†</sup>, Matthew C. Zwier<sup>2</sup>, Carsen A. Stringer<sup>3</sup>, Sundar Raman Subramanian<sup>1</sup>, Lillian T. Chong<sup>2</sup>, and Daniel M. Zuckerman<sup>1\*</sup>

## Supporting Information

1. Department of Computational and Systems Biology, University of Pittsburgh
2. Department of Chemistry, University of Pittsburgh
3. College of Arts and Sciences, University of Pittsburgh

† Equal contributions

\* Corresponding author: ddmmzz@pitt.edu

February 25, 2014

### S1. Reference coordinates for the order parameters in Ala4

For Ala4, two sets of reference coordinates were used on each dimension. In the first dimension, the set of  $N = 5$  torsions  $\{\phi_2, \psi_2, \phi_3, \psi_3, \phi_4\}$  were measured and a dihedral distance  $D = \sqrt{\frac{1}{N} \sum_i d_i^2} \in [0, 180]$  is used with respect to the reference values  $\{-83.9, 166.8, -48.7, -43.7, -54.0\}$ , where  $d_i$  is the circular distance between the current value of the  $i$ -th angle and our reference, i.e., the smaller of the two arclengths along the circumference. Those reference values were chosen in order to have a good separation of states (see Fig. 3 in the main document).

In the second dimension, a regular RMSD, using only heavy atoms, is measured with respect to the following structure given in PDB format.

|        |    |     |     |   |                                             |        |       |      |      |
|--------|----|-----|-----|---|---------------------------------------------|--------|-------|------|------|
| REMARK | 1  |     |     |   | PDB file used as reference in 2nd dimension |        |       |      |      |
| ATOM   | 1  | N   | ALA | 1 | 1.705                                       | -0.670 | 6.305 | 0.00 | 0.00 |
| ATOM   | 2  | H1  | ALA | 1 | 1.470                                       | -0.554 | 5.330 | 0.00 | 0.00 |
| ATOM   | 3  | H2  | ALA | 1 | 0.936                                       | -0.333 | 6.867 | 0.00 | 0.00 |
| ATOM   | 4  | H3  | ALA | 1 | 2.060                                       | -1.605 | 6.444 | 0.00 | 0.00 |
| ATOM   | 5  | CA  | ALA | 1 | 2.848                                       | 0.235  | 6.617 | 0.00 | 0.00 |
| ATOM   | 6  | HA  | ALA | 1 | 2.592                                       | 0.962  | 7.388 | 0.00 | 0.00 |
| ATOM   | 7  | CB  | ALA | 1 | 4.035                                       | -0.597 | 7.105 | 0.00 | 0.00 |
| ATOM   | 8  | HB1 | ALA | 1 | 4.309                                       | -1.323 | 6.340 | 0.00 | 0.00 |
| ATOM   | 9  | HB2 | ALA | 1 | 4.883                                       | 0.059  | 7.303 | 0.00 | 0.00 |
| ATOM   | 10 | HB3 | ALA | 1 | 3.760                                       | -1.121 | 8.021 | 0.00 | 0.00 |
| ATOM   | 11 | C   | ALA | 1 | 3.236                                       | 1.010  | 5.363 | 0.00 | 0.00 |
| ATOM   | 12 | O   | ALA | 1 | 2.963                                       | 0.576  | 4.243 | 0.00 | 0.00 |
| ATOM   | 13 | N   | ALA | 2 | 3.877                                       | 2.159  | 5.556 | 0.00 | 0.00 |
| ATOM   | 14 | H   | ALA | 2 | 4.068                                       | 2.489  | 6.491 | 0.00 | 0.00 |
| ATOM   | 15 | CA  | ALA | 2 | 4.300                                       | 2.985  | 4.432 | 0.00 | 0.00 |
| ATOM   | 16 | HA  | ALA | 2 | 3.459                                       | 3.174  | 3.764 | 0.00 | 0.00 |
| ATOM   | 17 | CB  | ALA | 2 | 4.830                                       | 4.326  | 4.942 | 0.00 | 0.00 |
| ATOM   | 18 | HB1 | ALA | 2 | 5.678                                       | 4.154  | 5.605 | 0.00 | 0.00 |
| ATOM   | 19 | HB2 | ALA | 2 | 5.148                                       | 4.937  | 4.097 | 0.00 | 0.00 |
| ATOM   | 20 | HB3 | ALA | 2 | 4.042                                       | 4.845  | 5.488 | 0.00 | 0.00 |
| ATOM   | 21 | C   | ALA | 2 | 5.385                                       | 2.280  | 3.627 | 0.00 | 0.00 |
| ATOM   | 22 | O   | ALA | 2 | 5.377                                       | 2.312  | 2.395 | 0.00 | 0.00 |
| ATOM   | 23 | N   | ALA | 3 | 6.317                                       | 1.642  | 4.328 | 0.00 | 0.00 |
| ATOM   | 24 | H   | ALA | 3 | 6.297                                       | 1.654  | 5.338 | 0.00 | 0.00 |
| ATOM   | 25 | CA  | ALA | 3 | 7.404                                       | 0.930  | 3.666 | 0.00 | 0.00 |
| ATOM   | 26 | HA  | ALA | 3 | 7.981                                       | 1.614  | 3.043 | 0.00 | 0.00 |
| ATOM   | 27 | CB  | ALA | 3 | 8.337                                       | 0.316  | 4.711 | 0.00 | 0.00 |
| ATOM   | 28 | HB1 | ALA | 3 | 7.776                                       | -0.378 | 5.337 | 0.00 | 0.00 |
| ATOM   | 29 | HB2 | ALA | 3 | 9.144                                       | -0.219 | 4.209 | 0.00 | 0.00 |
| ATOM   | 30 | HB3 | ALA | 3 | 8.757                                       | 1.106  | 5.333 | 0.00 | 0.00 |
| ATOM   | 31 | C   | ALA | 3 | 6.852                                       | -0.170 | 2.764 | 0.00 | 0.00 |
| ATOM   | 32 | O   | ALA | 3 | 7.249                                       | -0.294 | 1.606 | 0.00 | 0.00 |
| ATOM   | 33 | N   | ALA | 4 | 5.934                                       | -0.966 | 3.304 | 0.00 | 0.00 |
| ATOM   | 34 | H   | ALA | 4 | 5.647                                       | -0.841 | 4.264 | 0.00 | 0.00 |
| ATOM   | 35 | CA  | ALA | 4 | 5.335                                       | -2.053 | 2.539 | 0.00 | 0.00 |
| ATOM   | 36 | HA  | ALA | 4 | 6.104                                       | -2.751 | 2.209 | 0.00 | 0.00 |
| ATOM   | 37 | CB  | ALA | 4 | 4.328                                       | -2.809 | 3.406 | 0.00 | 0.00 |
| ATOM   | 38 | HB1 | ALA | 4 | 3.546                                       | -2.125 | 3.736 | 0.00 | 0.00 |
| ATOM   | 39 | HB2 | ALA | 4 | 3.882                                       | -3.616 | 2.825 | 0.00 | 0.00 |

|      |    |     |     |   |       |        |       |      |      |
|------|----|-----|-----|---|-------|--------|-------|------|------|
| ATOM | 40 | HB3 | ALA | 4 | 4.837 | -3.226 | 4.275 | 0.00 | 0.00 |
| ATOM | 41 | C   | ALA | 4 | 4.634 | -1.510 | 1.297 | 0.00 | 0.00 |
| ATOM | 42 | O   | ALA | 4 | 4.769 | -2.062 | 0.205 | 0.00 | 0.00 |
| ATOM | 43 | OXT | ALA | 4 | 3.885 | -0.426 | 1.473 | 0.00 | 0.00 |

## S2. Visualization of the states used in Ala4 (A1, A2, B1 and B2)

In the main document, we showed the definition of the states used in the system Ala4. Here we show representative structures of them.

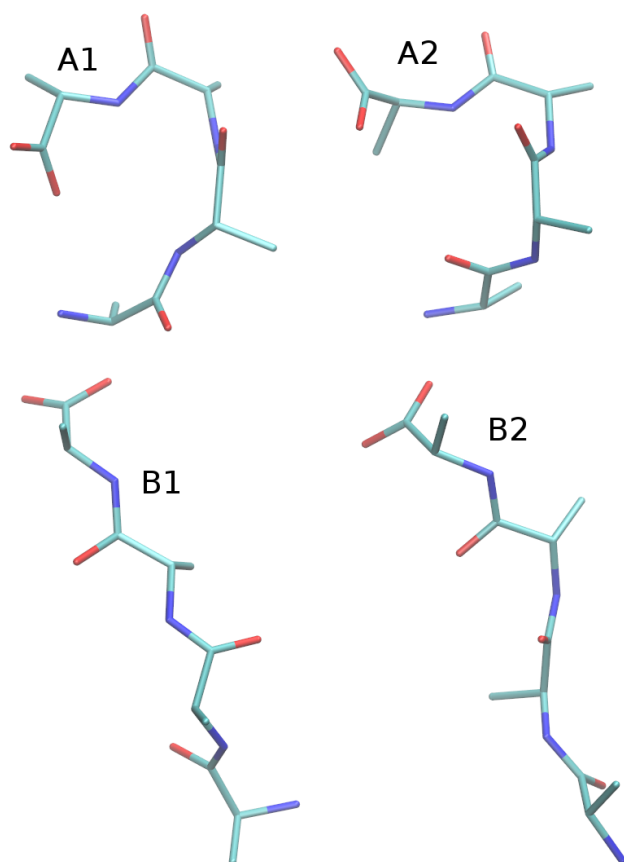

Figure 1: Representative structures for the states A1, A2, B1 and B2.

### S3. Maximum likelihood estimation reversible Markov State Models )

The next figure shows that the regular Markovian approach, in our methane system, even if it is improved by a more realistic model where the flux matrix is symmetric [J. Chem. Theory Comput. 2011, 7, 3412], is still biased. This is not surprising, since the our WE simulation was long enough to overcome any low sampling issue that may be improved by a better estimation.

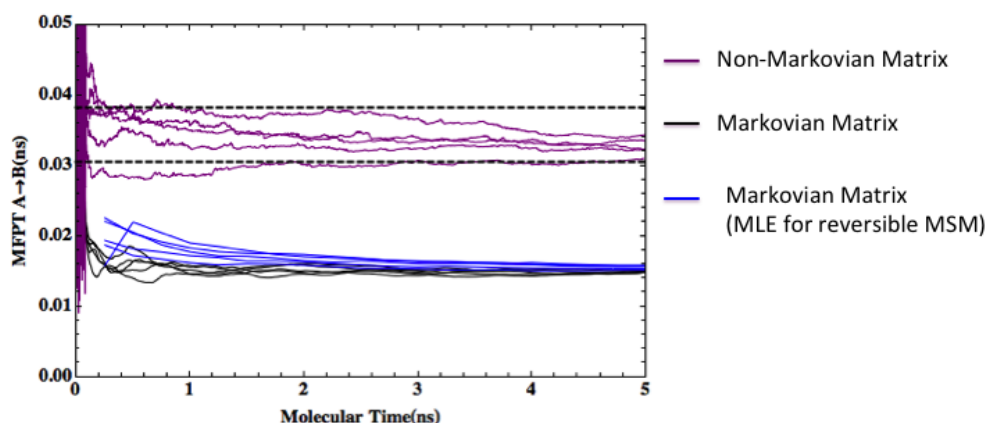

Figure 2: Markovian, non-Markovian and Maximum Likelihood for reversible Markov State Models estimates for mean first passage times (MFPTs) from  $A(r < 5\text{\AA})$  to  $B(r > 11\text{\AA})$  are plotted vs. molecular time. Five independent WE runs are shown, each based on 0.4 s of total simulation time. Dashed lines indicate roughly a 95% confidence interval based on 0.4 s of brute force simulation. Each ns of molecular time corresponds to approximately 80 ns of WE simulation accounting for all trajectories in a single run.
